# Supplementary material for: Layer-dependent optically-induced spin polarization in InSe
Source: arXiv:2212.05423 ancillary file (2022-12-11)
Supplement: Supplementary file 1 [file Nelson2022_InSe_Supplemental.pdf]

# Supplemental Material: Layer-dependent optically-induced spin polarization in InSe

Jovan Nelson[1], Teodor K. Stanev[2], Dmitry Lebedev[3], Trevor LaMountain[1], J. Tyler Gish[3], Hongfei Zeng[2], Hyeondeok Shin[4], Olle Heinonen[5,6], Kenji Watanabe[7], Takashi Taniguchi[8], Mark C. Hersam[1,3, 9, 10], and Nathaniel P. Stern[1,2]

[1]*Applied Physics Program, Northwestern University, Evanston, Illinois 60208, United States*
[2]*Department of Physics and Astronomy, Northwestern University, Evanston, Illinois 60208, United States*
[3]*Department of Material Science & Engineering, Northwestern University, Evanston, Illinois 60208, United States*
[4]*Computational Science Division, Argonne National Laboratory, Lemont, Illinois 60439, United States*
[5]*Material Science Division, Argonne National Laboratory, Lemont, Illinois 60439, United States*
[6]*Present and permanent address: Seagate Technology, 7801 Computer Ave, Bloomington, Minnesota 55435, United States*
[7]*Research Center for Functional Materials, National Institute for Materials Science, 1-1 Namiki, Tsukuba 305-0044, Japan*
[8]*International Center for Materials Nanoarchitectonics, National Institute for Materials Science, 1-1 Namiki, Tsukuba 305-0044, Japan*
[9]*Department of Chemistry, Northwestern University, Evanston, Illinois 60208, United States*
[10]*Department of Electrical Engineering and Computer Science, Northwestern University, Evanston, Illinois 60208, United States*

December 9, 2022

# 1. Characterizing InSe polytype

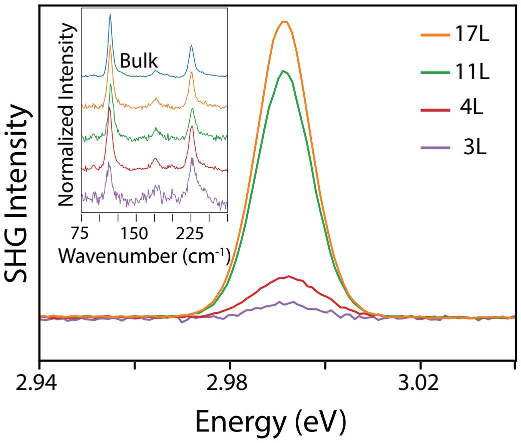


**Figure S1:** Second harmonic generation (SHG) is present in InSe of odd and even layer number. Each sample was pumped by 1.49 eV pulsed laser. This is evidence that these InSe samples are non-centrosymmetric. Inset shows Raman measurements done with 2.33 eV pump for each thickness.

An important detail to consider when studying layered group-III monochalogenides is polytypism. Polytypes differ by stacking order, and even small differences in layer alignments can lead to interesting properties in InSe. Novel effects such as sizable spin splitting [1, 2] and ferroelecticity [3, 4] have either been predicted or experimentally verified for specific polytypes. However, due to the similarities of common polytpes ($\epsilon$, $\gamma$, $\beta$), clearly identifying them can be challenging. Mechanical exfoliation can also introduce lattice defects, potentially creating further uncertainty.

There are few different experimental techniques that have been used to determine the polytype of exfoliated InSe, namely electron diffraction and microscopy [5, 6], Raman spectroscopy [6–11], and second harmonic generation (SHG) [6, 7]. Often multiple techniques and modeling are needed to determine accurately which stacking order is being examined [5, 6]. For the work presented here, the stacking configuration is important because it determines whether the system is centrosymmetric or non-centrosymmetric. A non-centrosymmetric system has a sizable spin splitting induced by symmetry-dependent SOC. The system then can be influenced by the Dresselhaus effect which influences spin dynamics [1, 2].

Here we apply SHG and Raman techniques in order to determine the polytype of InSe. Due to SHG being a non-linear effect that occurs in non-centorsymmetric systems, observing it in our samples, will give further evidence that the Dresselhaus effect is present in the system (therefore the poltype will most likely be $\delta$, $\epsilon$. $\gamma$, or odd layers of $\beta$). In figure S1, SHG is shown. This is generated by a pulsed pump laser at 1.49 eV (830 nm). Regardless of thickness (or layer number) there is a SHG signal, indicating that our crystal structure is always non-centrosymmetric. Comparing SHG and the Raman for different layers with those in the literature [6–11], our samples are most likely $\epsilon$-InSe.

## 2. InSe flakes

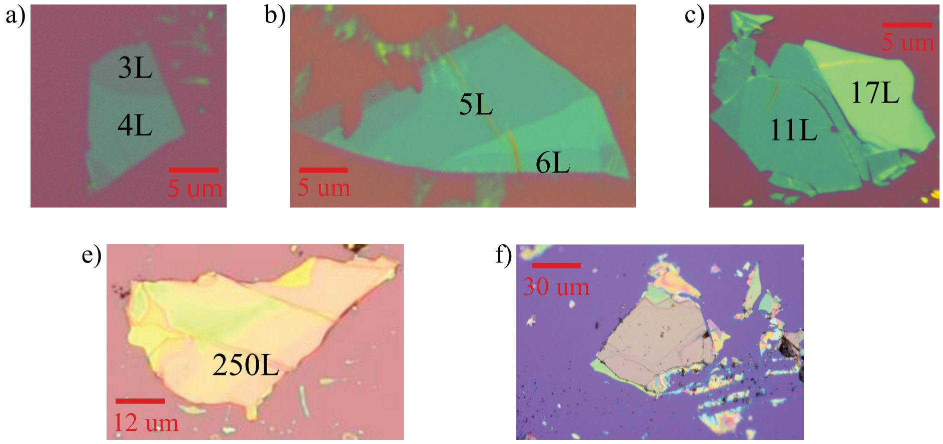


**Figure S2:** The InSe flakes measured can be seen in images a) - f). Although thin flakes are encapsulated when measurements were performed, here images for bare InSe flakes are presented for clarity. For a) - e), the general regions measured are labeled with their respective layer number. These flakes were measured using the polarized PL measurement scheme shown in figure S3 (right). f) is the bulk flake measured using TRKR and TR depicted in Fig. S4 (right).

# 3. Polarized photoluminescence

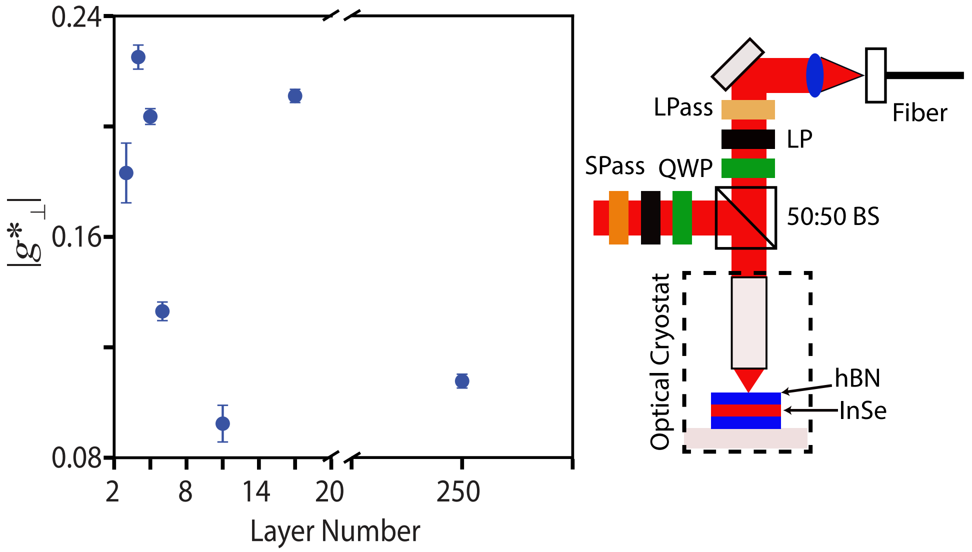


**Figure S3:** Left image is the extracted effective $g$-factor from polarized PL measurement for different thicknesses. Right image is a layout of the polarized PL setup. To reduce pump laser noise, a shortpass (SPass) and longpass (LPass) are put on the input and output, respectively. On the collection side, the fiber leads to a spectrometer.

The general optics setup for the polarized PL setup can be seen in figure S3. On the input side, there is a shorpass filter (SPass), linear polarizer (LP), and quarter-wave plate (QWP). The then circular or linear polarized beam passes through a 50:50 beamspliter (BS) into an objective inside of an attoDRY2100 magneto-optical cryostat. The beam reflected from the sample then passes through circular polarized collection optics (a QWP and LP) and is filtered with a longpass filter (LPass) before being focused onto a fiber that leads to a 750 mm spectrometer with a CCD camera (Andor). For the CW laser system used in these experiments, there is a dead zone between 660 nm (1.87 eV) and 700 nm (1.77 eV). The experimental setup has a characterized uniform $\sim$4% offset in the raw polarization which is subtracted from reported $P$ calculations.

Using the 9 T superconducting magnetic in the Attodry system, we performed magneto-PL measurements shown in the main text. The extracted values for the effective $g$-factorare shown in the left image in figure S3.

# 4. Modeling $P$ with layer-dependent spin relaxation

In order to qualitatively model degree of circular polarization, $P$, with layer number, we look to work done in Ref. [12], where $\alpha$, the strength of SOC can be described as:

$$\alpha(\epsilon_z, N) = \alpha_D + \alpha_R \approx \alpha_\infty \left(1 - \frac{\chi}{(N + 2.84)^2}\right) \pm \epsilon_z \eta(N) \tag{S1}$$

The first term models the layer dependence of the Dresselhaus ($\alpha_D$) effect while the second term models the layer and electric field ($\epsilon_z$) dependence of the Rashba effect ($\alpha_R$). For the first term, the constants $\alpha_\infty = 34.5$ meVÅ and $\chi = 14.9$ account for SOC strength at the conduction band edge for a 3D bulk InSe and the nonlinear dependence of bulk SOC. In the second term, $\eta(N)$ is a slope relating $\alpha$ to $\epsilon_z$ which contains the $N$ dependence of the Rashba term [12]. This equation can be used to reflect the Dyakonov-Perel (DP) relaxation of spins in the system. Assuming the system is in the motional narrowing regime, spin relaxation can be described as $1/\tau_s = \Omega^2 \tau_p$, where $\tau_s$ is the spin lifetime, $\Omega$ the spin precession due to SOC, and $\tau_p$ is the scattering momentum time [13]. $\Omega$ is $\Omega = \alpha k_f$ where $k_f$ is the Fermi momentum [12]. With this, we can plug in Eq. S1 into the DP relationship of $\Omega$ to $\tau_s$.

$$1/\tau_s(\epsilon_z, N) \approx \tau_p k_f^2 \left(\alpha_\infty \left(1 - \frac{\chi}{(N + 2.84)^2}\right) \pm \epsilon_z \eta(N)\right)^2 \tag{S2}$$

It can be assumed that the carrier density is similar for different thickness, as they are all derived from the same n-type crystal, temperature is constant, and no external electrical gate is applied. Therefore, in this qualitative model, we can assume $k_f$ is a constant, $\tau_p$ is a constant, and $\epsilon_z = 0$. Therefore we are left with just the Dresselhaus term and a constant A that contains $k_f$ and $\tau_p$. Therefore it can be rewritten as:

$$1/\tau_s(N) \approx A\alpha_D^2(N) \tag{S3}$$

This can inserted into Eq. 1 in the main text which is a rate equation used to calculate $P$. The full layer-dependent expression takes the form of:

$$P(N) = \frac{P_0}{1 + \tau_r A \alpha_D^2(N)} \tag{S4}$$

where $\tau_r$ is the recombination lifetime estimated by time-resolved measurement.

## 5. Time-resolved measurements

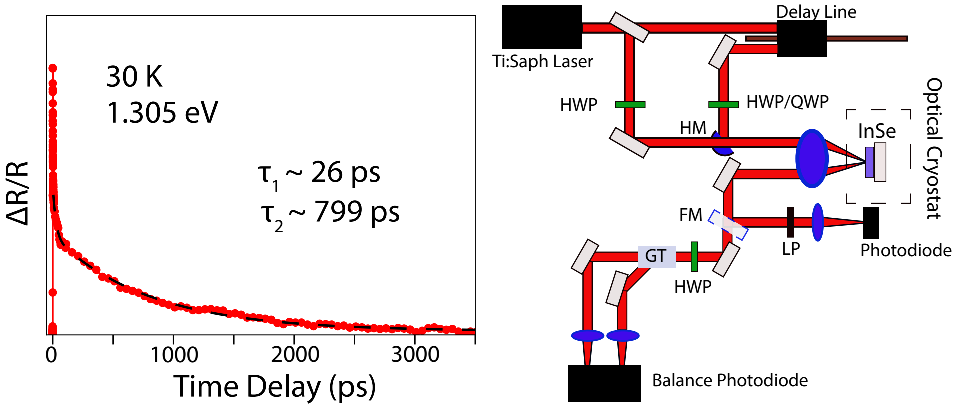


**Figure S4:** Left image is the transient reflectance (TR) for bulk InSe near the band edge. The right image is a diagram of the time-resolved set up. FM (flip mirror) is used to switch between a single photodiode for TR and balanced photodiode for time-resolved Kerr Rotation (TRKR). For the pump, a HWP is used for TR and a QWP is used for TRKR measurements.

Time resolved measurements were conducted with a tunable 76 MHz Ti:Sapphire laser. A 50:50 plate beamsplitter is used to create a pump and probe beam. The pump time separation from the probe is controlled by a mechanical delay line. A wave plate is used to adjust polarization before incident on a half mirror (HM). The HM allows the pump to be aligned parallel to the probe beam but spatially separated by 1-inch. The InSe sample was measured in a Quantum Design OptiCool, which has a temperature range of 1.7 K - 350 K and a magnetic field up to 7 T. The distance from the outside window of this cryostat to the center is roughly ∼15 cm. A two inch lens with focal length of 15 cm is used to focus the beams onto our samples which are 3 - 4 cm from the center of the cryostat. The field here deviates less than 1% from the set value. In this Voigt geometry configuration with this cryostat, pump and probe pulses have beam sizes of 65 $\mu$m and 30 $\mu$m, respectively. In order to optimize the signal with this large spot, a large flake is used ($\geq$ 500 nm ).

After the beams are reflected off the sample, they are either directed to a single photodiode or balanced phototdiodes using a flip mounted mirror. The single photodiode is used for transient reflectance (TR) measurements while the balanced photodiodes are used for time-resolved Kerr rotation (TRKR). For TR, a half-wave plate (HWP) is used to cross polarize the pump with respect to the probe. In the path of the single photodiode, a linear polarizer (LP) is oriented to filter out any pump scatter. For TRKR, a quarter-wave plate (QWP) is used to adjust curricular polarization of the pump. The FM is flipped down and the beams travel through a HWP and Glan-Thompson (GT) polarizer. For both measurement schemes, the pump is chopped at 100 kHz and the probe is demodulated with a lockin amplifier. To reduce noise in TRKR measurements, the probe is also chopped at 1 kHz and the 100 kHz demodulation is fed into a second demodulator at 1 kHz to filter out unintended signal from pump scatter.

Using a one-color pump-probe scheme, TR was measured near the band edge for InSe

with a thickness $\geq$ 500 nm. Three time scales are apparent. The initial relaxation is very fast and thus the data are characterized by a double exponential fit for times greater than 5 ps. The exciton lifetime ($\tau_2$) is 799 $\pm$ 24 ps.

## 6. Calculating effective $g$-factor from the band model

As described in the main text, the $\boldsymbol{k} \cdot \boldsymbol{p}$ perturbation theory Hamiltonian and hopping model for InSe multilayers developed in Ref. [14] was used to calculate the effective $g$-factor for different layer numbers. This was done by plugging in the matrix elements at the center of the bands into the expression for the Landé effective $g$-factor derived from $\boldsymbol{k} \cdot \boldsymbol{p}$ theory [15]:

$$\frac{g_k^*}{g_0} - 1 = \frac{1}{im_0} \sum_u \frac{\langle k|p_x|u\rangle\langle u|p_y|k\rangle - \langle k|p_y|u\rangle\langle u|p_x|k\rangle}{E_k - E_u} \tag{S5}$$

where $g_0 = 2$, $m_0$ is the free electron mass, $k$ is the band in which the effective $g$-factor is calculated, $E_k$ is the energy of band $k$, and $u$ denotes a band at energy $E_u$. $p_x$ and $p_y$ are the x and y components of the momentum operator. This calculates the orbital $g$-factor of the selected $k$ band.

# References


[1] Li, P. & Appelbaum, I. Symmetry, distorted band structure, and spin-orbit coupling of group-III metal-monochalcogenide monolayers. *Physical Review B - Condensed Matter and Materials Physics* **92**, 1–12 (2015).

[2] Do, D. T., Mahanti, S. D. & Lai, C. W. Spin splitting in 2D monochalcogenide semiconductors. *Scientific Reports* **5**, 17044 (2015).

[3] Liu, L. *et al.* Ferroelectric-Gated InSe Photodetectors with High On/Off Ratios and Photoresponsivity. *Nano Letters* **20**, 6666–6673 (2020).

[4] Zheng, C. *et al.* Room temperature in-plane ferroelectricity in van der Waals $In_2Se_3$. *Science Advances* **4**, eaar7720 (2018).

[5] Bergeron, H. *et al.* Large-area optoelectronic-grade InSe thin films via controlled phase evolution. *Applied Physics Reviews* **7** (2020).

[6] Hao, Q. *et al.* Phase Identification and Strong Second Harmonic Generation in Pure $\epsilon$-InSe and Its Alloys. *Nano Letters* **19**, 2634–2640 (2019).

[7] Huang, W., Gan, L., Li, H., Ma, Y. & Zhai, T. Phase-Engineered Growth of Ultrathin InSe Flakes by Chemical Vapor Deposition for High-Efficiency Second Harmonic Generation. *Chemistry - A European Journal* **24**, 15678–15684 (2018).

[8] Sánchez-Royo, J. F. *et al.* Electronic structure, optical properties, and lattice dynamics in atomically thin indium selenide flakes. *Nano Research* **7**, 1556–1568 (2014).

[9] Wu, M. *et al.* Crystal structure and optical performance in bulk $\gamma$-InSe single crystals. *AIP Advances* **9**, 025013 (2019).

[10] Tamalampudi, S. R. *et al.* Thickness-Dependent Resonant Raman and E Photoluminescence Spectra of Indium Selenide and Indium Selenide Graphene Heterostructures. *Journal of Physical Chemistry C* **123**, 15345–15353 (2019).

[11] Molas, M. R. *et al.* Raman spectroscopy of gase and inse post-transition metal chalcogenides layers. *Faraday Discuss.* **227**, 163–170 (2021).

[12] Ceferino, A. *et al.* Tunable spin-orbit coupling in two-dimensional InSe. *Physical Review B* **104**, 1–21 (2021).

[13] Wu, M. W., Jiang, J. H. & Weng, M. Q. Spin dynamics in semiconductors. *Physics Reports* **493**, 61–236 (2010).

[14] Magorrian, S. J., Zólyomi, V. & Fal'ko, V. I. Spin-orbit coupling, optical transitions, and spin pumping in monolayer and few-layer InSe. *Physical Review B* **96**, 195428 (2017).

[15] Hermann, C. & Weisbuch, C. $k \cdot p$ perturbation theory in III-V compounds and alloys: a reexamination. *Physical Review B* **15**, 823–833 (1977).
